# Supplementary material for: Design of a mobile neutron spectrometer for the Laboratori Nazionali del Gran Sasso (LNGS)
Source: arXiv:2307.06660 source file (2023-11-07)
Supplement: Supplementary file 1 [file appendix.tex]

\appendix
\section{Appendix title}
Please always give a title also for appendices.
